# Supplementary material for: How Do Viewers Synthesize Conflicting Information from Data Visualizations?
Source: arXiv:2208.03828 source file (2022-08-07)
Supplement: Supplementary file 1 [file SupplmentaryMaterials.tex]

\documentclass{article}
\usepackage[utf8]{inputenc}
\usepackage{cite}
%\raggedbottom
\usepackage[bottom]{footmisc}
\usepackage{mathptmx}
\usepackage{graphicx}
\usepackage{siunitx}
\usepackage{times}
\usepackage[T1]{fontenc}
\usepackage[latin1]{inputenc}
\usepackage{enumitem}
\usepackage{wrapfig}
\usepackage{multirow}
\usepackage{adjustbox}
\usepackage{mwe}
\usepackage{graphbox}
\usepackage{dirtytalk}
\usepackage{soul}
% for highlighting
\usepackage{mdframed}
\usepackage{tabularx}
\usepackage{xcolor}
\usepackage{enumitem}
\usepackage{pdfpages}
\usepackage{dcolumn}
\usepackage[graphicx]{realboxes}
\usepackage{rotating}
\usepackage{longtable}
\usepackage{hyperref}

\title{Supplmentary Materials}
\author{Submission ID \# 1103}
\date{March 2022}

\begin{document}

\maketitle

\begin{table}[!htbp] \centering 
  \caption{Summary statistics} 
  \label{} 
\begin{tabular}{@{\extracolsep{5pt}} cccc} 
\\[-1.8ex]\hline 
\hline \\[-1.8ex] 
Experiment & N & $\mu_{Age}$ & $\sigma_{Age}$ \\ 
\hline \\[-1.8ex] 
Experiment 1 & 294 & 34.81 & 12.67 \\ 
Experiment 2A & 281 & 42.26 & 14.85\\ 
Experiment 2B & 287 & 42.64 & 14.61 \\ 
Experiment 3 & 279 & 38.75 & 13.25 \\ 
\hline \\[-1.8ex] 
\end{tabular} 
\end{table}

% Table created by stargazer v.5.2.3 by Marek Hlavac, Social Policy Institute. E-mail: marek.hlavac at gmail.com
% Date and time: Sun, Apr 17, 2022 - 23:16:06
\begin{table}[!htbp] \centering 
  \caption{Summary Statistics by Education levels} 
  \label{} 
\begin{tabular}{@{\extracolsep{5pt}} ccccc} 
\\[-1.8ex]\hline 
\hline \\[-1.8ex] 
Experiment & education & N & $\mu_{Age}$ & $\sigma_{Age}$ \\ 
\hline \\[-1.8ex] 
Experiment 1 & Associate-degree & 25 & 38.76 & 14.94 \\ 
Experiment 1 & Bachelors  & 103 & 33.58 & 8.82 \\ 
Experiment 1 & Doctorate & 2 & 58.5 & 3.54 \\ 
Experiment 1 & Eighth grade & 1 & 23 & NA \\ 
Experiment 1 & High School & 36 & 29.97 & 10.56 \\ 
Experiment 1 & Masters & 39 & 42.87 & 16.084 \\ 
Experiment 1 & Professional degree & 7 & 38 & 11.80 \\ 
Experiment 1 & Some college credit & 67 & 30.36 & 10.87 \\ 
Experiment 1 & Some schooling & 5 & 31 & 5.1 \\ 
Experiment 1 & Vocational & 9 & 51.22& 16.36\\ 
\hline 
Experiment 2A & Associate-degree & 19 & 41.58 & 12.70 \\ 
Experiment 2A & Bachelors  & 111 & 44.35 & 13.69 \\ 
Experiment 2A & Doctorate & 3 & 56.67 & 15.95 \\ 
Experiment 2A & Eighth grade & 1 & 57 & NA \\ 
Experiment 2A & High School & 30 & 36.43 & 15.22 \\ 
Experiment 2A & Masters & 47 & 46 & 15.83 \\ 
Experiment 2A & Professional degree & 3 & 58.67 & 4.73\\ 
Experiment 2A & Some college credit & 58 & 36.24 & 14.44 \\ 
Experiment 2A & Some schooling & 2 & 27 & 2.83 \\ 
Experiment 2A & Vocational & 7 & 49.57 & 11.21 \\ 
\hline 
Experiment 2B & Associate-degree & 23 & 41.48 & 11.41 \\ 
Experiment 2B & Bachelors  & 113 & 41.84 & 14.14\\ 
Experiment 2B & Doctorate & 9 & 46.22 & 14.22\\ 
Experiment 2B & High School & 26 & 38.5 & 14.12 \\ 
Experiment 2B & Masters & 57 & 45.89 & 13.83 \\ 
Experiment 2B & Professional degree & 9 & 49.44 & 13.73\\ 
Experiment 2B & Some college credit & 44 & 40.20 & 17.94 \\ 
Experiment 2B & Some schooling & 1 & 49 & NA \\ 
Experiment 2B & Vocational & 5 & 51.8 & 13.55 \\ 
\hline 
Experiment 3 & Associate-degree & 18 & 40.78 & 12.35\\ 
Experiment 3 & Bachelors  & 131 & 38.29& 13.10 \\ 
Experiment 3 & Doctorate & 2 & 52 & 8.49 \\ 
Experiment 3 & High School & 26 & 34.58 & 12.88 \\ 
Experiment 3 & Masters & 50 & 39.8 & 11.23\\ 
Experiment 3 & Professional degree & 6 & 45 & 14.51 \\ 
Experiment 3 & Some college credit & 40 & 38.08 & 16.15\\ 
Experiment 3 & Vocational & 6 & 45.83 & 12.19\\ 
\hline \\[-1.8ex] 
\end{tabular} 
\end{table}

\begin{table}[!htbp] \centering 
  \caption{t-tests between response slopes(widget) and priors} 
  \label{} 
  \rotatebox{90}{
\begin{tabular}{@{\extracolsep{5pt}} ccccccccc} 
\\[-1.8ex]\hline 

\hline \\[-1.8ex] 
Experiment & Condition & estimate & estimate1 & estimate2 & t - statistic & p\_value & method & alternative \\ 
\hline \\[-1.8ex] 
Experiment 2A & 1 & 0.132 & 0.424 & 0.292 & 2.658 &\textasteriskcentered \textasteriskcentered \textasteriskcentered  & Welch 2 Sample t-test & 2.sided \\ 
Experiment 2A & 2 & -0.6 & -0.262 & 0.338 & -9.709 &\textasteriskcentered \textasteriskcentered \textasteriskcentered  & Welch 2 Sample t-test & 2.sided \\ 
Experiment 2A & 3 & -0.052 & 0.243 & 0.295 & -0.753 & & Welch 2 Sample t-test & 2.sided \\ 
Experiment 2A & 4 & -0.103 & 0.208 & 0.311 & -1.692 &\textasteriskcentered  & Welch 2 Sample t-test & 2.sided \\ 
Experiment 2A & 5 & -0.064 & 0.246 & 0.31 & -1.142 & & Welch 2 Sample t-test & 2.sided \\ 
Experiment 2A & 6 & -0.374 & -0.047 & 0.326 & -6.015 &\textasteriskcentered \textasteriskcentered \textasteriskcentered  & Welch 2 Sample t-test & 2.sided \\ 
Experiment 2B & 1 & 0.053 & 0.419 & 0.366 & 1.124 & & Welch 2 Sample t-test & 2.sided \\ 
Experiment 2B & 2 & -0.557 & -0.187 & 0.37 & -9.423 &\textasteriskcentered \textasteriskcentered \textasteriskcentered  & Welch 2 Sample t-test & 2.sided \\ 
Experiment 2B & 3 & 0.081 & 0.375 & 0.294 & 1.409 & & Welch 2 Sample t-test & 2.sided \\ 
Experiment 2B & 4 & -0.055 & 0.278 & 0.333 & -0.889 & & Welch 2 Sample t-test & 2.sided \\ 
Experiment 2B & 5 & -0.055 & 0.339 & 0.394 & -1.242 & & Welch 2 Sample t-test & 2.sided \\ 
Experiment 2B & 6 & -0.332 & 0.02 & 0.352 & -5.394 &\textasteriskcentered \textasteriskcentered \textasteriskcentered  & Welch 2 Sample t-test & 2.sided \\ 
Experiment 3 & 1 & 0.041 & 0.394 & 0.354 & 1.084 & & Welch 2 Sample t-test & 2.sided \\ 
Experiment 3 & 2 & -0.629 & -0.268 & 0.361 & -8.938 &\textasteriskcentered \textasteriskcentered \textasteriskcentered  & Welch 2 Sample t-test & 2.sided \\ 
Experiment 3 & 3 & -0.009 & 0.343 & 0.352 & -0.116 & & Welch 2 Sample t-test & 2.sided \\ 
Experiment 3 & 4 & -0.115 & 0.272 & 0.387 & -2.114 &\textasteriskcentered \textasteriskcentered  & Welch 2 Sample t-test & 2.sided \\ 
Experiment 3 & 5 & -0.155 & 0.243 & 0.398 & -2.487 &\textasteriskcentered \textasteriskcentered  & Welch 2 Sample t-test & 2.sided \\ 
Experiment 3 & 6 & -0.329 & 0.075 & 0.404 & -6.03 &\textasteriskcentered \textasteriskcentered \textasteriskcentered  & Welch 2 Sample t-test & 2.sided \\ 

\hline 
\hline \\[-1.8ex] 
\textit{Note:}  & \multicolumn{1}{r}{$^{*}$p$<$0.1; $^{**}$p$<$0.05; $^{***}$p$<$0.01} \\ 
\end{tabular} }
\end{table}

%%%%%%%%%%%%%%%%%%%%%%%%%%%%%%%%%%%%%%%%%%%%%%%
%%%%%%%%%%%%%%%%%%%%%%%%%%%%%%%%%%%%%%%%%%%%%%%
\begin{table}[!htbp] \centering 
  \caption{t-test between widget response and average of stimuli slopes without considering Order effects} 
  \label{} 
\begin{tabular}{@{\extracolsep{5pt}} ccccccc} 
\\[-1.8ex]\hline 
\hline \\[-1.8ex] 
Experiment & Condition & estimate & estimate1 & estimate2 & t - statistic & p\_value \\ 
\hline \\[-1.8ex] 
Experiment 1 & 1 & -0.027 & 0.424 & 0.451 &  -0.94 &   \\ 
Experiment 1 & 2 & 0.14 & -0.276 & -0.416 &  3.611 & \textasteriskcentered \textasteriskcentered \textasteriskcentered   \\ 
Experiment 1 & 3 & 0.143 & 0.164 & 0.021 &  2.197 & \textasteriskcentered \textasteriskcentered   \\ 
Experiment 1 & 4 & -0.011 & 0.219 & 0.23 &  -0.312 &   \\ 
Experiment 1 & 5 & -0.038 & 0.251 & 0.289 &  -0.797 &   \\ 
Experiment 1 & 6 & 0.143 & -0.126 & -0.269 &  4.131 & \textasteriskcentered \textasteriskcentered \textasteriskcentered   \\ 
Experiment 2A & 1 & -0.027 & 0.424 & 0.451 &  -0.924 &   \\ 
Experiment 2A & 2 & 0.153 & -0.262 & -0.416 &  3.292 & \textasteriskcentered \textasteriskcentered \textasteriskcentered   \\ 
Experiment 2A & 3 & 0.222 & 0.243 & 0.021 &  4.073 & \textasteriskcentered \textasteriskcentered \textasteriskcentered   \\ 
Experiment 2A & 4 & -0.022 & 0.208 & 0.23 &  -0.519 &   \\ 
Experiment 2A & 5 & -0.042 & 0.246 & 0.289 &  -1.127 &   \\ 
Experiment 2A & 6 & 0.222 & -0.047 & -0.269 &  5.017 & \textasteriskcentered \textasteriskcentered \textasteriskcentered   \\ 
Experiment 2B & 1 & -0.032 & 0.419 & 0.451 &  -1.229 &   \\ 
Experiment 2B & 2 & 0.228 & -0.187 & -0.416 &  5.24 & \textasteriskcentered \textasteriskcentered \textasteriskcentered   \\ 
Experiment 2B & 3 & 0.354 & 0.375 & 0.021 &  9.077 & \textasteriskcentered \textasteriskcentered \textasteriskcentered   \\ 
Experiment 2B & 4 & 0.048 & 0.278 & 0.23 &  1.117 &   \\ 
Experiment 2B & 5 & 0.05 & 0.339 & 0.289 &  1.887 & \textasteriskcentered   \\ 
Experiment 2B & 6 & 0.29 & 0.02 & -0.269 &  5.963 & \textasteriskcentered \textasteriskcentered \textasteriskcentered   \\ 
Experiment 3 & 1 & -0.057 & 0.394 & 0.451 &  -2.593 & \textasteriskcentered \textasteriskcentered   \\ 
Experiment 3 & 2 & 0.148 & -0.268 & -0.416 &  2.982 & \textasteriskcentered \textasteriskcentered \textasteriskcentered   \\ 
Experiment 3 & 3 & 0.322 & 0.343 & 0.021 &  5.598 & \textasteriskcentered \textasteriskcentered \textasteriskcentered   \\ 
Experiment 3 & 4 & 0.042 & 0.272 & 0.23 &  1.135 &   \\ 
Experiment 3 & 5 & -0.046 & 0.243 & 0.289 &  -1.026 &   \\ 
Experiment 3 & 6 & 0.344 & 0.075 & -0.269 &  9.129 & \textasteriskcentered \textasteriskcentered \textasteriskcentered   \\ 

\hline 
\hline \\[-1.8ex] 
\textit{Note:}  & \multicolumn{1}{r}{$^{*}$p$<$0.1; $^{**}$p$<$0.05; $^{***}$p$<$0.01} \\ 
\end{tabular} 
\end{table} 

%%%%%%%%%%%%%%%%%%%%%%%%%%%%%%%%%%%%%%%%%%%%%%%
%%%%%%%%%%%%%%%%%%%%%%%%%%%%%%%%%%%%%%%%%%%%%%%
\begin{table}{}
  \caption{t-test between widget response and average of stimuli slopes with Order effects} 
  \label{} 

\begin{tabular}{@{\extracolsep{1pt}} ccccccc} 
\\[-1.8ex]\hline 
\hline \\[-1.8ex] 
Experiment & Condition & estimate & estimate1 & estimate2 & t - statistic & p\_value \\ 
\hline \\[-1.8ex] 
Experiment 1 & 11  -  High Pos and Med.Pos & -0.018 & 0.432 & 0.451 & -0.412 &  \\ 
Experiment 1 & 12  -  Med.Pos and High Pos & -0.037 & 0.413 & 0.451 & -1.065 &  \\ 
Experiment 1 & 21  -  High Neg and Med.Neg & 0.121 & -0.294 & -0.416 & 2.288 &\textasteriskcentered \textasteriskcentered   \\ 
Experiment 1 & 22  -  Med.Neg and High Neg & 0.167 & -0.248 & -0.416 & 2.944 &  \\ 
Experiment 1 & 31  -  High Neg and High Pos & -0.003 & 0.018 & 0.021 & -0.037 &  \\ 
Experiment 1 & 32  -  High Pos and High Neg & 0.276 & 0.297 & 0.021 & 3.345 &\textasteriskcentered \textasteriskcentered \textasteriskcentered   \\ 
Experiment 1 & 41  -  High Pos and Med.Neg & 0.014 & 0.245 & 0.23 & 0.255 &  \\ 
Experiment 1 & 42  -  Med.Neg and High Pos & -0.031 & 0.199 & 0.23 & -0.691 &  \\ 
Experiment 1 & 51  -  High Pos and Low Neg & -0.032 & 0.257 & 0.289 & -0.584 &  \\ 
Experiment 1 & 52  -  Low Neg and High Pos & -0.045 & 0.244 & 0.289 & -0.534 &  \\ 
Experiment 1 & 61  -  High Neg and Low Pos & 0.219 & -0.05 & -0.269 & 4.031 &\textasteriskcentered \textasteriskcentered \textasteriskcentered   \\ 
Experiment 1 & 62  -  Low Pos and High Neg & 0.072 & -0.197 & -0.269 & 1.785 &\textasteriskcentered   \\ 
Experiment 2A & 11  -  High Pos and Med.Pos & -0.025 & 0.426 & 0.451 & -0.585 &  \\ 
Experiment 2A & 12  -  Med.Pos and High Pos & -0.028 & 0.422 & 0.451 & -0.711 &  \\ 
Experiment 2A & 21  -  High Neg and Med.Neg & 0.206 & -0.21 & -0.416 & 2.975 &\textasteriskcentered \textasteriskcentered \textasteriskcentered   \\ 
Experiment 2A & 22  -  Med.Neg and High Neg & 0.081 & -0.335 & -0.416 & 1.49 &  \\ 
Experiment 2A & 31  -  High Neg and High Pos & 0.225 & 0.246 & 0.021 & 2.898 &  \\ 
Experiment 2A & 32  -  High Pos and High Neg & 0.219 & 0.24 & 0.021 & 2.812 &  \\ 
Experiment 2A & 41  -  High Pos and Med.Neg & 0.077 & 0.307 & 0.23 & 1.276 &  \\ 
Experiment 2A & 42  -  Med.Neg and High Pos & -0.121 & 0.11 & 0.23 & -2.322 &\textasteriskcentered \textasteriskcentered   \\ 
Experiment 2A & 51  -  High Pos and Low Neg & -0.008 & 0.281 & 0.289 & -0.203 &  \\ 
Experiment 2A & 52  -  Low Neg and High Pos & -0.105 & 0.184 & 0.289 & -1.39 &  \\ 
Experiment 2A & 61  -  High Neg and Low Pos & 0.397 & 0.128 & -0.269 & 9.187 &\textasteriskcentered \textasteriskcentered \textasteriskcentered   \\ 
Experiment 2A & 62  -  Low Pos and High Neg & 0.062 & -0.207 & -0.269 & 1.073 &  \\ 
Experiment 2B & 11  -  High Pos and Med.Pos & -0.012 & 0.439 & 0.451 & -0.295 &  \\ 
Experiment 2B & 12  -  Med.Pos and High Pos & -0.052 & 0.399 & 0.451 & -1.479 &  \\ 
Experiment 2B & 21  -  High Neg and Med.Neg & 0.245 & -0.17 & -0.416 & 3.752 &\textasteriskcentered \textasteriskcentered \textasteriskcentered   \\ 
Experiment 2B & 22  -  Med.Neg and High Neg & 0.215 & -0.2 & -0.416 & 3.633 &\textasteriskcentered \textasteriskcentered \textasteriskcentered   \\ 
Experiment 2B & 31  -  High Neg and High Pos & 0.249 & 0.27 & 0.021 & 4.084 &\textasteriskcentered \textasteriskcentered \textasteriskcentered   \\ 
Experiment 2B & 32  -  High Pos and High Neg & 0.41 & 0.432 & 0.021 & 8.667 &\textasteriskcentered \textasteriskcentered \textasteriskcentered   \\ 
Experiment 2B & 41  -  High Pos and Med.Neg & 0.049 & 0.28 & 0.23 & 0.844 &  \\ 
Experiment 2B & 42  -  Med.Neg and High Pos & 0.047 & 0.277 & 0.23 & 0.725 &  \\ 
Experiment 2B & 51  -  High Pos and Low Neg & 0.084 & 0.372 & 0.289 & 2.416 &\textasteriskcentered \textasteriskcentered   \\ 
Experiment 2B & 52  -  Low Neg and High Pos & 0.014 & 0.303 & 0.289 & 0.351 &  \\ 
Experiment 2B & 61  -  High Neg and Low Pos & 0.388 & 0.119 & -0.269 & 6.648 &\textasteriskcentered \textasteriskcentered \textasteriskcentered   \\ 
Experiment 2B & 62  -  Low Pos and High Neg & 0.199 & -0.07 & -0.269 & 2.762 &\textasteriskcentered \textasteriskcentered   \\ 
Experiment 3 & 11  -  High Pos and Med.Pos & -0.032 & 0.419 & 0.451 & -1.04 &  \\ 
Experiment 3 & 12  -  Med.Pos and High Pos & -0.075 & 0.376 & 0.451 & -2.465 &\textasteriskcentered \textasteriskcentered   \\ 
Experiment 3 & 21  -  High Neg and Med.Neg & 0.144 & -0.271 & -0.416 & 2.224 &\textasteriskcentered \textasteriskcentered   \\ 
Experiment 3 & 22  -  Med.Neg and High Neg & 0.153 & -0.263 & -0.416 & 1.927 &\textasteriskcentered   \\ 
Experiment 3 & 31  -  High Neg and High Pos & 0.458 & 0.479 & 0.021 & 6.274 &\textasteriskcentered \textasteriskcentered \textasteriskcentered   \\ 
Experiment 3 & 32  -  High Pos and High Neg & 0.242 & 0.263 & 0.021 & 3.111 &\textasteriskcentered \textasteriskcentered \textasteriskcentered   \\ 
Experiment 3 & 41  -  High Pos and Med.Neg & 0.089 & 0.319 & 0.23 & 1.937 &\textasteriskcentered   \\ 
Experiment 3 & 42  -  Med.Neg and High Pos & -0.012 & 0.218 & 0.23 & -0.21 &  \\ 
Experiment 3 & 51  -  High Pos and Low Neg & 0.047 & 0.336 & 0.289 & 0.612 &  \\ 
Experiment 3 & 52  -  Low Neg and High Pos & -0.111 & 0.178 & 0.289 & -2.19 &\textasteriskcentered \textasteriskcentered   \\ 
Experiment 3 & 61  -  High Neg and Low Pos & 0.331 & 0.062 & -0.269 & 5.98 &\textasteriskcentered \textasteriskcentered \textasteriskcentered   \\ 
Experiment 3 & 62  -  Low Pos and High Neg & 0.36 & 0.091 & -0.269 & 7.174 &\textasteriskcentered \textasteriskcentered \textasteriskcentered   \\ 

\hline 
\hline \\[-1.8ex] 
\textit{Note:}  & \multicolumn{1}{r}{$^{*}$p$<$0.1; $^{**}$p$<$0.05; $^{***}$p$<$0.01} \\ 
\end{tabular}
\end{table} 

%%%%%%%%%%%%%%%%%%%%%%%%%%%%%%%%%%%%
%%%%%%%%%%%%%%%%%%%%%%%%%%%%%%%%%%%%

\begin{table}[!htbp] \centering 
  \caption{Meaningfulness - distance from mathematical average} 
  \label{} 
\begin{tabular}{@{\extracolsep{5pt}} cccccc} 
\\[-1.8ex]\hline 
\hline \\[-1.8ex] 
Effect Size Cohen`s d & Experiment & Condition & n & magnitude \\ 
\hline \\[-1.8ex] 
 -0.138 & Experiment 1 & 1 & 46 & 1 \\ 
 0.557 & Experiment 1 & 2 & 42 & 3 \\ 
 0.331 & Experiment 1 & 3 & 44 & 2 \\ 
 -0.043 & Experiment 1 & 4 & 54 & 1 \\ 
 -0.113 & Experiment 1 & 5 & 50 & 1 \\ 
 0.542 & Experiment 1 & 6 & 58 & 3 \\ 
 -0.123 & Experiment 2A & 1 & 56 & 1 \\ 
 0.465 & Experiment 2A & 2 & 50 & 2 \\ 
 0.636 & Experiment 2A & 3 & 41 & 3 \\ 
 -0.080 & Experiment 2A & 4 & 42 & 1 \\ 
 -0.162 & Experiment 2A & 5 & 48 & 1 \\ 
 0.756 & Experiment 2A & 6 & 44 & 3 \\ 
 -0.179 & Experiment 2B & 1 & 47 & 1 \\ 
 0.733 & Experiment 2B & 2 & 51 & 3 \\ 
 1.435 & Experiment 2B & 3 & 40 & 4 \\ 
 0.156 & Experiment 2B & 4 & 51 & 1 \\ 
 0.256 & Experiment 2B & 5 & 54 & 2 \\ 
 0.898 & Experiment 2B & 6 & 44 & 4 \\ 
 -0.314 & Experiment 3 & 1 & 68 & 2 \\ 
 0.477 & Experiment 3 & 2 & 39 & 2 \\ 
 0.853 & Experiment 3 & 3 & 43 & 4 \\ 
 0.165 & Experiment 3 & 4 & 47 & 1 \\ 
 -0.164 & Experiment 3 & 5 & 39 & 1 \\ 
 1.392 & Experiment 3 & 6 & 43 & 4 \\ 

\hline 
\hline \\[-1.8ex] 
\textit{Note:}  & \multicolumn{1}{r}{$^{*}$p$<$0.1; $^{**}$p$<$0.05; $^{***}$p$<$0.01} \\ 
\end{tabular} 
\end{table}

%%%%%%%%%%%%%%%%%%%%%%%%%%%%%%%%%%%%%%%
%%%%%%%%%%%%%%%%%%%%%%%%%%%%%%%%%%%%%%%

\begin{table}[!htbp] \centering 
  \caption{Differences between response slopes computed through widgets and input boxes - considering order effects} 
  \label{} 
\begin{tabular}{@{\extracolsep{5pt}} cccccccc} 
\\[-1.8ex]\hline 
\hline \\[-1.8ex] 
Exp.& Condition & estimate & estimate1 & estimate2 & t - statistic & Signi. & p.value \\ 
\hline \\[-1.8ex] 
 1 & 11  -  High Pos + Med.Pos & -0.267 & 0.432 & 0.699 &  -3.807 & \textasteriskcentered \textasteriskcentered \textasteriskcentered  & 0  \\ 
 2A & 11  -  High Pos + Med.Pos & -0.292 & 0.426 & 0.718 &  -4.444 & \textasteriskcentered \textasteriskcentered \textasteriskcentered  & 0  \\ 
 2B & 11  -  High Pos + Med.Pos & -0.222 & 0.439 & 0.661 &  -3.804 & \textasteriskcentered \textasteriskcentered \textasteriskcentered  & 0  \\ 
 3 & 11  -  High Pos + Med.Pos & -0.222 & 0.419 & 0.64 &  -4.289 & \textasteriskcentered \textasteriskcentered \textasteriskcentered  & 0  \\ 
 1 & 12  -  Med.Pos + High Pos & -0.156 & 0.413 & 0.569 &  -1.797 & \textasteriskcentered  & 0.083  \\ 
 2A & 12  -  Med.Pos + High Pos & -0.261 & 0.422 & 0.684 &  -4.172 & \textasteriskcentered \textasteriskcentered \textasteriskcentered  & 0  \\ 
 2B & 12  -  Med.Pos + High Pos & -0.229 & 0.399 & 0.628 &  -4.155 & \textasteriskcentered \textasteriskcentered \textasteriskcentered  & 0  \\ 
 3 & 12  -  Med.Pos + High Pos & -0.197 & 0.376 & 0.573 &  -3.737 & \textasteriskcentered \textasteriskcentered \textasteriskcentered  & 0  \\ 
 1 & 21  -  High Neg + Med.Neg & 0.016 & -0.294 & -0.31 &  0.13 &  & 0.897  \\ 
 2A & 21  -  High Neg + Med.Neg & 0.03 & -0.21 & -0.24 &  0.216 &  & 0.83  \\ 
 2B & 21  -  High Neg + Med.Neg & 0.107 & -0.17 & -0.277 &  0.826 &  & 0.415  \\ 
 3 & 21  -  High Neg + Med.Neg & 0.155 & -0.271 & -0.426 &  1.258 &  & 0.216  \\ 
 1 & 22  -  Med.Neg + High Neg & 0.046 & -0.248 & -0.294 &  0.368 &  & 0.716  \\ 
 2A & 22  -  Med.Neg + High Neg & -0.062 & -0.335 & -0.273 &  -0.439 &  & 0.665  \\ 
 2B & 22  -  Med.Neg + High Neg & 0.284 & -0.2 & -0.484 &  2.93 & \textasteriskcentered \textasteriskcentered \textasteriskcentered  & 0.005  \\ 
 3 & 22  -  Med.Neg + High Neg & 0.108 & -0.263 & -0.371 &  0.708 &  & 0.485  \\ 
 1 & 31  -  High Neg + High Pos & 0.052 & 0.018 & -0.034 &  0.339 &  & 0.736  \\ 
 2A & 31  -  High Neg + High Pos & -0.098 & 0.246 & 0.344 &  -0.742 &  & 0.463  \\ 
 2B & 31  -  High Neg + High Pos & -0.23 & 0.27 & 0.5 &  -2.002 & \textasteriskcentered  & 0.058  \\ 
 3 & 31  -  High Neg + High Pos & -0.293 & 0.479 & 0.772 &  -3.116 & \textasteriskcentered \textasteriskcentered \textasteriskcentered  & 0.004  \\ 
 1 & 32  -  High Pos + High Neg & -0.071 & 0.297 & 0.369 &  -0.542 &  & 0.591  \\ 
 2A & 32  -  High Pos + High Neg & 0.048 & 0.24 & 0.192 &  0.361 &  & 0.72  \\ 
 2B & 32  -  High Pos + High Neg & -0.092 & 0.432 & 0.523 &  -1.098 &  & 0.278  \\ 
 3 & 32  -  High Pos + High Neg & -0.083 & 0.263 & 0.346 &  -0.635 &  & 0.528  \\ 
 1 & 41  -  High Pos + Med.Neg & -0.127 & 0.245 & 0.372 &  -1.101 &  & 0.278  \\ 
 2A & 41  -  High Pos + Med.Neg & -0.201 & 0.307 & 0.508 &  -2.246 & \textasteriskcentered \textasteriskcentered  & 0.03  \\ 
 2B & 41  -  High Pos + Med.Neg & -0.155 & 0.28 & 0.435 &  -1.414 &  & 0.165  \\ 
 3 & 41  -  High Pos + Med.Neg & -0.245 & 0.319 & 0.564 &  -3.042 & \textasteriskcentered \textasteriskcentered \textasteriskcentered  & 0.004  \\ 
 1 & 42  -  Med.Neg + High Pos & -0.03 & 0.199 & 0.229 &  -0.294 &  & 0.77  \\ 
 2A & 42  -  Med.Neg + High Pos & -0.242 & 0.11 & 0.352 &  -2.991 & \textasteriskcentered \textasteriskcentered \textasteriskcentered  & 0.005  \\ 
 2B & 42  -  Med.Neg + High Pos & -0.2 & 0.277 & 0.477 &  -1.956 & \textasteriskcentered  & 0.057  \\ 
 3 & 42  -  Med.Neg + High Pos & -0.164 & 0.218 & 0.382 &  -1.764 & \textasteriskcentered  & 0.085  \\ 
 1 & 51  -  High Pos + Low Neg & -0.211 & 0.257 & 0.467 &  -2.161 & \textasteriskcentered \textasteriskcentered  & 0.036  \\ 
 2A & 51  -  High Pos + Low Neg & -0.262 & 0.281 & 0.542 &  -3.531 & \textasteriskcentered \textasteriskcentered \textasteriskcentered  & 0.001  \\ 
 2B & 51  -  High Pos + Low Neg & -0.194 & 0.372 & 0.566 &  -3.585 & \textasteriskcentered \textasteriskcentered \textasteriskcentered  & 0.001  \\ 
 3 & 51  -  High Pos + Low Neg & -0.155 & 0.336 & 0.492 &  -1.232 &  & 0.228  \\ 
 1 & 52  -  Low Neg + High Pos & -0.276 & 0.244 & 0.52 &  -2.171 & \textasteriskcentered \textasteriskcentered  & 0.036  \\ 
 2A & 52  -  Low Neg + High Pos & -0.211 & 0.184 & 0.395 &  -1.709 & \textasteriskcentered  & 0.098  \\ 
 2B & 52  -  Low Neg + High Pos & -0.26 & 0.303 & 0.563 &  -4.115 & \textasteriskcentered \textasteriskcentered \textasteriskcentered  & 0  \\ 
 3 & 52  -  Low Neg + High Pos & -0.074 & 0.178 & 0.252 &  -0.773 &  & 0.444  \\ 
 1 & 61  -  High Neg + Low Pos & -0.014 & -0.05 & -0.036 &  -0.143 &  & 0.887  \\ 
 2A & 61  -  High Neg + Low Pos & -0.063 & 0.128 & 0.191 &  -0.732 &  & 0.469  \\ 
 2B & 61  -  High Neg + Low Pos & -0.041 & 0.119 & 0.16 &  -0.425 &  & 0.673  \\ 
 3 & 61  -  High Neg + Low Pos & -0.002 & 0.062 & 0.064 &  -0.019 &  & 0.985  \\ 
 1 & 62  -  Low Pos + High Neg & -0.045 & -0.197 & -0.152 &  -0.429 &  & 0.67  \\ 
 2A & 62  -  Low Pos + High Neg & 0.121 & -0.207 & -0.328 &  1.087 &  & 0.284  \\ 
 2B & 62  -  Low Pos + High Neg & 0.03 & -0.07 & -0.1 &  0.225 &  & 0.823  \\ 
 3 & 62  -  Low Pos + High Neg & 0.003 & 0.091 & 0.088 &  0.024 &  & 0.981  \\ 

\hline 
\hline \\[-1.8ex] 
\textit{Note:}  & \multicolumn{1}{r}{$^{*}$p$<$0.1; $^{**}$p$<$0.05; $^{***}$p$<$0.01} \\ 
\end{tabular} 
\end{table} 

%%%%%%%%%%%%%%%%%%%%%%%%%%%%%%%%%%%%%%%%%%%%%%%%%%%
%%%%%%%%%%%%%%%%%%%%%%%%%%%%%%%%%%%%%%%%%%%%%%%%%%%

\begin{table}[!htbp] \centering 
  \caption{Differences between estimation of y values at x = 20 through widget and input boxes} 
  \label{} 
\begin{tabular}{@{\extracolsep{5pt}} ccccccc} 
\\[-1.8ex]\hline 
\hline \\[-1.8ex] 
Experiment & estimate & estimate1 & estimate2 & t - statistic & Signi. & p.value  \\ 
\hline \\[-1.8ex] 
Experiment 1 & 2.324 & 43.273 & 40.949 &  1.795 & \textasteriskcentered  & 0.073  \\ 
Experiment 2A & 3.242 & 43.786 & 40.544 &  2.447 & \textasteriskcentered \textasteriskcentered  & 0.015  \\ 
Experiment 2B & 0.233 & 40.414 & 40.181 &  0.19 &  & 0.849  \\ 
Experiment 3 & 1.453 & 41.475 & 40.022 &  1.142 &  & 0.254  \\ 

\hline 
\hline \\[-1.8ex] 
\textit{Note:}  & \multicolumn{1}{r}{$^{*}$p$<$0.1; $^{**}$p$<$0.05; $^{***}$p$<$0.01} \\ 
\end{tabular} 
\end{table}

\begin{table}[!htbp] \centering 
  \caption{Differences between estimation of y values at x = 20 through widget and input boxes - considering different conditions} 
  \label{} 
\begin{tabular}{@{\extracolsep{5pt}} ccccccc} 
\\[-1.8ex]\hline 
\hline \\[-1.8ex] 
Experiment & Condition & estimate & estimate1 & estimate2 & t - statistic & p\_value\\ 
\hline \\[-1.8ex] 
Experiment 1 & 1 & 4.788 & 35.918 & 31.13 &  2.206 &\textasteriskcentered \textasteriskcentered  \\ 
Experiment 1 & 2 & 0.283 & 54.688 & 54.405 &  0.084 & \\ 
Experiment 1 & 3 & -0.181 & 40.501 & 40.682 &  -0.048 & \\ 
Experiment 1 & 4 & 1.058 & 39.076 & 38.019 &  0.434 & \\ 
Experiment 1 & 5 & 4.596 & 38.836 & 34.24 &  1.901 &\textasteriskcentered  \\ 
Experiment 1 & 6 & 2.967 & 50.674 & 47.707 &  1.054 & \\ 
Experiment 2A & 1 & 7.055 & 36.805 & 29.75 &  3.193 &\textasteriskcentered \textasteriskcentered \textasteriskcentered  \\ 
Experiment 2A & 2 & -0.586 & 55.534 & 56.12 &  -0.181 & \\ 
Experiment 2A & 3 & 2.152 & 41.25 & 39.098 &  0.628 & \\ 
Experiment 2A & 4 & 4.854 & 39.949 & 35.095 &  2.217 &\textasteriskcentered \textasteriskcentered  \\ 
Experiment 2A & 5 & 5.813 & 39.418 & 33.604 &  2.59 &\textasteriskcentered \textasteriskcentered  \\ 
Experiment 2A & 6 & -0.59 & 50.114 & 50.705 &  -0.188 & \\ 
Experiment 2B & 1 & 2.636 & 33.742 & 31.106 &  1.539 & \\ 
Experiment 2B & 2 & -7.174 & 53.375 & 60.549 &  -2.517 &\textasteriskcentered \textasteriskcentered  \\ 
Experiment 2B & 3 & 2.474 & 34.974 & 32.5 &  0.983 & \\ 
Experiment 2B & 4 & 1.68 & 36.621 & 34.941 &  0.711 & \\ 
Experiment 2B & 5 & 2.711 & 36.526 & 33.815 &  1.69 &\textasteriskcentered  \\ 
Experiment 2B & 6 & -0.506 & 46.63 & 47.136 &  -0.173 & \\ 
Experiment 3 & 1 & 3.869 & 37.031 & 33.162 &  2.242 &\textasteriskcentered \textasteriskcentered  \\ 
Experiment 3 & 2 & -7.489 & 53.562 & 61.051 &  -2.474 &\textasteriskcentered \textasteriskcentered  \\ 
Experiment 3 & 3 & 5.506 & 37.809 & 32.302 &  1.547 & \\ 
Experiment 3 & 4 & 3.996 & 37.634 & 33.638 &  1.581 & \\ 
Experiment 3 & 5 & 2.397 & 41.397 & 39 &  0.766 & \\ 
Experiment 3 & 6 & -1.944 & 45.474 & 47.419 &  -0.79 & \\ 

\hline 
\hline \\[-1.8ex] 
\textit{Note:}  & \multicolumn{1}{r}{$^{*}$p$<$0.1; $^{**}$p$<$0.05; $^{***}$p$<$0.01} \\ 
\end{tabular} 
\end{table}

%%%%%%%%%%%%%%%%%%%%%%%%%%%%%%%%%%%%%%%%%%%%%%%%%
%%%%%%%%%%%%%%%%%%%%%%%%%%%%%%%%%%%%%%%%%%%%%%%%%

\begin{table}[!htbp] \centering 
  \caption{Differences between estimation of y values at x = 80 through widget and input boxes} 
  \label{} 
\begin{tabular}{@{\extracolsep{5pt}} ccccccc} 
\\[-1.8ex]\hline 
\hline \\[-1.8ex] 
Experiment & estimate & estimate1 & estimate2 & t - statistic & Signi. & p\_value  \\ 
\hline \\[-1.8ex] 
Experiment 1 & -3.174 & 49.846 & 53.02 &  -2.014 & 0.045 & \textasteriskcentered \textasteriskcentered   \\ 
Experiment 2A & -4.497 & 52.133 & 56.63 &  -3.073 & 0.002 & \textasteriskcentered \textasteriskcentered \textasteriskcentered   \\ 
Experiment 2B & -5.413 & 52.646 & 58.059 &  -4.003 & 0 & \textasteriskcentered \textasteriskcentered \textasteriskcentered   \\ 
Experiment 3 & -4.92 & 53.643 & 58.563 &  -3.39 & 0.001 & \textasteriskcentered \textasteriskcentered \textasteriskcentered   \\ 

\hline 
\hline \\[-1.8ex] 
\textit{Note:}  & \multicolumn{1}{r}{$^{*}$p$<$0.1; $^{**}$p$<$0.05; $^{***}$p$<$0.01} \\ 
\end{tabular} 
\end{table}

\begin{table}[!htbp] \centering 
  \caption{Differences between estimation of y values at x = 80 through widget and input boxes - considering different conditions} 
  \label{} 
\begin{tabular}{@{\extracolsep{5pt}} ccccccc} 
\\[-1.8ex]\hline 
\hline \\[-1.8ex] 
Experiment & S1 & estimate & estimate1 & estimate2 & t-statistic & p\_value \\ 
\hline \\[-1.8ex] 
Experiment 1 & 1 & -8.182 & 61.34 & 69.522 &  -3.282 & \textasteriskcentered \textasteriskcentered \textasteriskcentered  \\ 
Experiment 1 & 2 & 1.955 & 38.145 & 36.19 &  0.57 &  \\ 
Experiment 1 & 3 & -0.94 & 50.332 & 51.273 &  -0.215 &  \\ 
Experiment 1 & 4 & -3.342 & 52.232 & 55.574 &  -1.035 &  \\ 
Experiment 1 & 5 & -9.68 & 53.92 & 63.6 &  -2.719 & \textasteriskcentered \textasteriskcentered \textasteriskcentered  \\ 
Experiment 1 & 6 & 1.153 & 43.102 & 41.948 &  0.379 &  \\ 
Experiment 2A & 1 & -9.527 & 62.241 & 71.768 &  -4.322 & \textasteriskcentered \textasteriskcentered \textasteriskcentered  \\ 
Experiment 2A & 2 & -1.09 & 39.79 & 40.88 &  -0.324 &  \\ 
Experiment 2A & 3 & 0.986 & 55.84 & 54.854 &  0.298 &  \\ 
Experiment 2A & 4 & -8.432 & 52.449 & 60.881 &  -2.68 & \textasteriskcentered \textasteriskcentered \textasteriskcentered  \\ 
Experiment 2A & 5 & -8.816 & 54.205 & 63.021 &  -2.781 & \textasteriskcentered \textasteriskcentered \textasteriskcentered  \\ 
Experiment 2A & 6 & 1.392 & 47.278 & 45.886 &  0.431 &  \\ 
Experiment 2B & 1 & -10.892 & 58.853 & 69.745 &  -5.33 & \textasteriskcentered \textasteriskcentered \textasteriskcentered  \\ 
Experiment 2B & 2 & 5.266 & 42.128 & 36.863 &  1.686 & \textasteriskcentered  \\ 
Experiment 2B & 3 & -5.926 & 57.474 & 63.4 &  -1.874 & \textasteriskcentered  \\ 
Experiment 2B & 4 & -8.947 & 53.327 & 62.275 &  -3.071 & \textasteriskcentered \textasteriskcentered \textasteriskcentered  \\ 
Experiment 2B & 5 & -10.814 & 56.871 & 67.685 &  -5.597 & \textasteriskcentered \textasteriskcentered \textasteriskcentered  \\ 
Experiment 2B & 6 & -0.747 & 47.844 & 48.591 &  -0.245 &  \\ 
Experiment 3 & 1 & -8.572 & 60.678 & 69.25 &  -4.555 & \textasteriskcentered \textasteriskcentered \textasteriskcentered  \\ 
Experiment 3 & 2 & 0.639 & 37.485 & 36.846 &  0.172 &  \\ 
Experiment 3 & 3 & -4.154 & 58.404 & 62.558 &  -0.996 &  \\ 
Experiment 3 & 4 & -8.413 & 53.949 & 62.362 &  -2.656 &  \\ 
Experiment 3 & 5 & -4.044 & 55.981 & 60.026 &  -1.33 &  \\ 
Experiment 3 & 6 & -1.93 & 49.953 & 51.884 &  -0.664 &  \\ 

\hline 
\hline \\[-1.8ex] 
\textit{Note:}  & \multicolumn{1}{r}{$^{*}$p$<$0.1; $^{**}$p$<$0.05; $^{***}$p$<$0.01} \\ 
\end{tabular} 
\end{table}

%%%%%%%%%%%%%%%%%%%%%%%%%%%%%%%%%%%%
%%%%%%%%%%%%%%%%%%%%%%%%%%%%%%%%%%%%

\begin{table}[] \centering 
  \caption{Agreement statistics for the decision task between various input methods\\} 
  \label{} 
  \rotatebox[]{90}{

\begin{tabular}{ @{}cccccccc} 
\\[-1.8ex]\hline 
\hline \\[-1.8ex] 
Experiment & Condition & Average-Widget & Average-Text & Average-Decision & Widget-Text & Widget-Decision & Text-Decision \\ 
\hline \\[-1.8ex] 
 1 & 11  -  High Pos and Medium Pos & 1 & 0.84 & 0.92 & 0.84 & 0.92 & 0.84 \\ 
 1 & 12  -  Medium Pos and High Pos & 1 & 1 & 1 & 1 & 1 & 1 \\ 
 1 & 21  -  High Neg and Medium Neg & 0 & 0 & 0.8 & 1 & 0.2 & 0.2 \\ 
 1 & 22  -  Medium Neg and High Neg & 0 & 0 & 0.75 & 1 & 0.25 & 0.25 \\ 
 1 & 31  -  High Neg and High Pos & 1 & 0.95 & 0.71 & 0.95 & 0.71 & 0.76 \\ 
 1 & 32  -  High Pos and High Neg & 1 & 1 & 0.65 & 1 & 0.65 & 0.65 \\ 
 1 & 41  -  High Pos and Medium Neg & 1 & 0.96 & 0.83 & 0.96 & 0.83 & 0.88 \\ 
 1 & 42  -  Medium Neg and High Pos & 1 & 0.97 & 0.7 & 0.97 & 0.7 & 0.67 \\ 
 1 & 51  -  High Pos and Low Neg & 1 & 0.97 & 0.83 & 0.97 & 0.83 & 0.79 \\ 
 1 & 52  -  Low Neg and High Pos & 1 & 0.9 & 0.75 & 0.9 & 0.75 & 0.65 \\ 
 1 & 61  -  High Neg and Low Pos & 0 & 0 & 0.52 & 1 & 0.48 & 0.48 \\ 
 1 & 62  -  Low Pos and High Neg & 0 & 0.03 & 0.77 & 0.97 & 0.23 & 0.2 \\ 
 2A & 11  -  High Pos and Medium Pos & 1 & 0.81 & 0.85 & 0.81 & 0.85 & 0.74 \\ 
 2A & 12  -  Medium Pos and High Pos & 1 & 0.9 & 0.86 & 0.9 & 0.86 & 0.83 \\ 
 2A & 21  -  High Neg and Medium Neg & 0 & 0.03 & 0.72 & 0.97 & 0.28 & 0.24 \\ 
 2A & 22  -  Medium Neg and High Neg & 0 & 0.05 & 0.67 & 0.95 & 0.33 & 0.29 \\ 
 2A & 31  -  High Neg and High Pos & 1 & 1 & 0.74 & 1 & 0.74 & 0.74 \\ 
 2A & 32  -  High Pos and High Neg & 1 & 0.95 & 0.77 & 0.95 & 0.77 & 0.73 \\ 
 2A & 41  -  High Pos and Medium Neg & 1 & 1 & 0.67 & 1 & 0.67 & 0.67 \\ 
 2A & 42  -  Medium Neg and High Pos & 1 & 1 & 0.76 & 1 & 0.76 & 0.76 \\ 
 2A & 51  -  High Pos and Low Neg & 1 & 0.9 & 0.87 & 0.9 & 0.87 & 0.77 \\ 
 2A & 52  -  Low Neg and High Pos & 1 & 1 & 0.71 & 1 & 0.71 & 0.71 \\ 
 2A & 61  -  High Neg and Low Pos & 0 & 0 & 0.52 & 1 & 0.48 & 0.48 \\ 
 2A & 62  -  Low Pos and High Neg & 0 & 0 & 0.57 & 1 & 0.43 & 0.43 \\ 
 2B & 11  -  High Pos and Medium Pos & 1 & 0.96 & 1 & 0.96 & 1 & 0.96 \\ 
 2B & 12  -  Medium Pos and High Pos & 1 & 1 & 1 & 1 & 1 & 1 \\ 
 2B & 21  -  High Neg and Medium Neg & 0 & 0 & 0.68 & 1 & 0.32 & 0.32 \\ 
 2B & 22  -  Medium Neg and High Neg & 0 & 0 & 0.76 & 1 & 0.24 & 0.24 \\ 
 2B & 31  -  High Neg and High Pos & 1 & 0.93 & 0.79 & 0.93 & 0.79 & 0.86 \\ 
 2B & 32  -  High Pos and High Neg & 1 & 1 & 0.85 & 1 & 0.85 & 0.85 \\ 
 2B & 41  -  High Pos and Medium Neg & 1 & 0.92 & 0.81 & 0.92 & 0.81 & 0.73 \\ 
 2B & 42  -  Medium Neg and High Pos & 1 & 0.96 & 0.84 & 0.96 & 0.84 & 0.8 \\ 
 2B & 51  -  High Pos and Low Neg & 1 & 1 & 0.96 & 1 & 0.96 & 0.96 \\ 
 2B & 52  -  Low Neg and High Pos & 1 & 1 & 0.81 & 1 & 0.81 & 0.81 \\ 
 2B & 61  -  High Neg and Low Pos & 0 & 0 & 0.29 & 1 & 0.71 & 0.71 \\ 
 2B & 62  -  Low Pos and High Neg & 0 & 0 & 0.35 & 1 & 0.65 & 0.65 \\ 

\hline \\[-1.8ex]
\end{tabular}}
\end{table} 

\begin{table}[] \centering 
  \caption{Agreement statistics for the decision task between various input methods - \textit{continued}\\} 
  \label{} 
  \rotatebox[]{90}{

\begin{tabular}{@{}cccccccc} 
\\[-1.8ex]\hline 
\hline \\[-1.8ex] 
 Experiment & Condition & Average-Widget & Average-Text & Average-Decision & Widget-Text & Widget-Decision & Text-Decision \\ 
\hline \\[-1.8ex] 

 3 & 11  -  High Pos and Medium Pos & 1 & 0.97 & 0.97 & 0.97 & 0.97 & 0.93 \\ 
 3 & 12  -  Medium Pos and High Pos & 1 & 0.92 & 0.95 & 0.92 & 0.95 & 0.87 \\ 
 3 & 21  -  High Neg and Medium Neg & 0 & 0 & 0.91 & 1 & 0.09 & 0.09 \\ 
 3 & 22  -  Medium Neg and High Neg & 0 & 0 & 0.81 & 1 & 0.19 & 0.19 \\ 
 3 & 31  -  High Neg and High Pos & 1 & 0.94 & 1 & 0.94 & 1 & 0.94 \\ 
 3 & 32  -  High Pos and High Neg & 1 & 1 & 0.74 & 1 & 0.74 & 0.74 \\ 
 3 & 41  -  High Pos and Medium Neg & 1 & 1 & 0.92 & 1 & 0.92 & 0.92 \\ 
 3 & 42  -  Medium Neg and High Pos & 1 & 0.95 & 0.82 & 0.95 & 0.82 & 0.77 \\ 
 3 & 51  -  High Pos and Low Neg & 1 & 1 & 0.88 & 1 & 0.88 & 0.88 \\ 
 3 & 52  -  Low Neg and High Pos & 1 & 1 & 0.7 & 1 & 0.7 & 0.7 \\ 
 3 & 61  -  High Neg and Low Pos & 0 & 0 & 0.29 & 1 & 0.71 & 0.71 \\ 
 3 & 62  -  Low Pos and High Neg & 0 & 0 & 0.37 & 1 & 0.63 & 0.63 \\ 
 \hline
  \hline \\[-1.8ex] 
 1 && 0.66 & 0.63 & 0.77 & 0.96 & 0.63 & 0.61 \\ 

 2A && 0.67 & 0.63 & 0.74 & 0.95 & 0.65 & 0.62 \\ 

 2B && 0.67 & 0.65 & 0.77 & 0.98 & 0.75 & 0.74 \\ 

 3 && 0.71 & 0.68 & 0.79 & 0.98 & 0.74 & 0.72 \\ 

\hline \\[-1.8ex]
\end{tabular}}
\end{table}

\begin{table}[!htbp] \centering 
  \caption{Effect of having a strong slope} 
  \label{} 
\begin{tabular}{@{\extracolsep{5pt}}lD{.}{.}{-3} } 
\\[-1.8ex]\hline 
\hline \\[-1.8ex] 
 & \multicolumn{1}{c}{\textit{Dependent variable:}} \\ 
\cline{2-2} 
\\[-1.8ex] & \multicolumn{1}{c}{Distance from mathematical average} \\ 
\hline \\[-1.8ex] 
 High Positive Slope & 0.048^{*} \\ 
  & (0.026) \\ 
  High Negative Slope & 0.268^{***} \\ 
  & (0.025) \\ 
  Experiment & 0.026 \\ 
  & (0.024) \\ 
  Experiment - 2B & 0.101^{***} \\ 
  & (0.023) \\ 
  Experiment - 3 & 0.062^{***} \\ 
  & (0.023) \\ 
  Constant & -0.106^{***} \\ 
  & (0.032) \\ 
 \hline \\[-1.8ex] 
Observations & \multicolumn{1}{c}{1,133} \\ 
R$^{2}$ & \multicolumn{1}{c}{0.163} \\ 
Adjusted R$^{2}$ & \multicolumn{1}{c}{0.159} \\ 
\hline 
\hline \\[-1.8ex] 
\textit{Note:}  & \multicolumn{1}{r}{$^{*}$p$<$0.1; $^{**}$p$<$0.05; $^{***}$p$<$0.01} \\ 
\end{tabular} 
\end{table}

\begin{table}[!htbp] \centering 
  \caption{Effect of having a strong slope - Experiment 1} 
  \label{} 
\begin{tabular}{@{\extracolsep{5pt}}lD{.}{.}{-3} } 
\\[-1.8ex]\hline 
\hline \\[-1.8ex] 
 & \multicolumn{1}{c}{\textit{Dependent variable:}} \\ 
\cline{2-2} 
\\[-1.8ex] & \multicolumn{1}{c}{Distance from mathematical average} \\ 
\hline \\[-1.8ex] 
 High Positive Slope & 0.001 \\ 
  & (0.053) \\ 
  High Negative Slope & 0.168^{***} \\ 
  & (0.051) \\ 
  Constant & -0.026 \\ 
  & (0.058) \\ 
 \hline \\[-1.8ex] 
Observations & \multicolumn{1}{c}{294} \\ 
R$^{2}$ & \multicolumn{1}{c}{0.075} \\ 
Adjusted R$^{2}$ & \multicolumn{1}{c}{0.069} \\ 
\hline 
\hline \\[-1.8ex] 
\textit{Note:}  & \multicolumn{1}{r}{$^{*}$p$<$0.1; $^{**}$p$<$0.05; $^{***}$p$<$0.01} \\ 
\end{tabular} 
\end{table} 

\begin{table}[!htbp] \centering 
  \caption{Effect of having a strong slope - Experiment 2A} 
  \label{} 
\begin{tabular}{@{\extracolsep{5pt}}lD{.}{.}{-3} } 
\\[-1.8ex]\hline 
\hline \\[-1.8ex] 
 & \multicolumn{1}{c}{\textit{Dependent variable:}} \\ 
\cline{2-2} 
\\[-1.8ex] & \multicolumn{1}{c}{Distance from mathematical average} \\ 
\hline \\[-1.8ex] 
 High Positive Slope & 0.023 \\ 
  & (0.054) \\ 
  High Negative Slope & 0.239^{***} \\ 
  & (0.051) \\ 
  Constant & -0.049 \\ 
  & (0.059) \\ 
 \hline \\[-1.8ex] 
Observations & \multicolumn{1}{c}{277} \\ 
R$^{2}$ & \multicolumn{1}{c}{0.133} \\ 
Adjusted R$^{2}$ & \multicolumn{1}{c}{0.127} \\ 
\hline 
\hline \\[-1.8ex] 
\textit{Note:}  & \multicolumn{1}{r}{$^{*}$p$<$0.1; $^{**}$p$<$0.05; $^{***}$p$<$0.01} \\ 
\end{tabular} 
\end{table}

\begin{table}[!htbp] \centering 
  \caption{Effect of having a strong slope - Experiment 2B} 
  \label{} 
\begin{tabular}{@{\extracolsep{5pt}}lD{.}{.}{-3} } 
\\[-1.8ex]\hline 
\hline \\[-1.8ex] 
 & \multicolumn{1}{c}{\textit{Dependent variable:}} \\ 
\cline{2-2} 
\\[-1.8ex] & \multicolumn{1}{c}{Distance from mathematical average} \\ 
\hline \\[-1.8ex] 
 High Positive Slope & 0.094^{*} \\ 
  & (0.049) \\ 
  High Negative Slope & 0.320^{***} \\ 
  & (0.046) \\ 
  Constant & -0.060 \\ 
  & (0.053) \\ 
 \hline \\[-1.8ex] 
Observations & \multicolumn{1}{c}{284} \\ 
R$^{2}$ & \multicolumn{1}{c}{0.203} \\ 
Adjusted R$^{2}$ & \multicolumn{1}{c}{0.197} \\ 
\hline 
\hline \\[-1.8ex] 
\textit{Note:}  & \multicolumn{1}{r}{$^{*}$p$<$0.1; $^{**}$p$<$0.05; $^{***}$p$<$0.01} \\ 
\end{tabular} 
\end{table}

\begin{table}[!htbp] \centering 
  \caption{Effect of having a strong slope - Experiment 3} 
  \label{} 
\begin{tabular}{@{\extracolsep{5pt}}lD{.}{.}{-3} } 
\\[-1.8ex]\hline 
\hline \\[-1.8ex] 
 & \multicolumn{1}{c}{\textit{Dependent variable:}} \\ 
\cline{2-2} 
\\[-1.8ex] & \multicolumn{1}{c}{Distance from mathematical average} \\ 
\hline \\[-1.8ex] 
 High Positive Slope & 0.073 \\ 
  & (0.053) \\ 
  High Negative Slope & 0.346^{***} \\ 
  & (0.048) \\ 
  Constant & -0.097^{*} \\ 
  & (0.057) \\ 
 \hline \\[-1.8ex] 
Observations & \multicolumn{1}{c}{278} \\ 
R$^{2}$ & \multicolumn{1}{c}{0.227} \\ 
Adjusted R$^{2}$ & \multicolumn{1}{c}{0.222} \\ 
\hline 
\hline \\[-1.8ex] 
\textit{Note:}  & \multicolumn{1}{r}{$^{*}$p$<$0.1; $^{**}$p$<$0.05; $^{***}$p$<$0.01} \\ 
\end{tabular} 
\end{table}

%%%%%%%%%%%%%%%%%%%%%%%%%%%%%%%%
%%%%%%%%%%%%%%%%%%%%%%%%%%%%%%%%

\begin{table}[!htbp] \centering 
  \caption{Effect of order of presentation of stronger slope on responses's distance from the stronger slope} 
  \label{} 
\begin{tabular}{@{\extracolsep{5pt}}lD{.}{.}{-3} } 
\\[-1.8ex]\hline 
\hline \\[-1.8ex] 
 & \multicolumn{1}{c}{\textit{Dependent variable:}} \\ 
\cline{2-2} 
\\[-1.8ex] & \multicolumn{1}{c}{Distance from greater slope} \\ 
\hline \\[-1.8ex] 
 Second slope is greater & 0.015 \\ 
  & (0.029) \\ 
  Constant & 0.600^{***} \\ 
  & (0.020) \\ 
 \hline \\[-1.8ex] 
Observations & \multicolumn{1}{c}{1,133} \\ 
R$^{2}$ & \multicolumn{1}{c}{0.0003} \\ 
Adjusted R$^{2}$ & \multicolumn{1}{c}{-0.001} \\ 
\hline 
\hline \\[-1.8ex] 
\textit{Note:}  & \multicolumn{1}{r}{$^{*}$p$<$0.1; $^{**}$p$<$0.05; $^{***}$p$<$0.01} \\ 
\end{tabular} 
\end{table} 

\begin{table}[!htbp] \centering 
  \caption{Effect of order of presentation of stronger slope on response's distance from the stronger slope - by experiment} 
  \label{} 
\begin{tabular}{@{\extracolsep{5pt}}lD{.}{.}{-3} } 
\\[-1.8ex]\hline 
\hline \\[-1.8ex] 
 & \multicolumn{1}{c}{\textit{Dependent variable:}} \\ 
\cline{2-2} 
\\[-1.8ex] & \multicolumn{1}{c}{Distance from stronger slope} \\ 
\hline \\[-1.8ex] 
 Second slope is stronger & 0.016 \\ 
  & (0.029) \\ 
  Experiment - 2A & 0.022 \\ 
  & (0.041) \\ 
  Experiment - 2B & 0.015 \\ 
  & (0.041) \\ 
  Experiment - 3 & 0.025 \\ 
  & (0.041) \\ 
  Constant & 0.584^{***} \\ 
  & (0.032) \\ 
 \hline \\[-1.8ex] 
Observations & \multicolumn{1}{c}{1,133} \\ 
R$^{2}$ & \multicolumn{1}{c}{0.001} \\ 
Adjusted R$^{2}$ & \multicolumn{1}{c}{-0.003} \\ 
\hline 
\hline \\[-1.8ex] 
\textit{Note:}  & \multicolumn{1}{r}{$^{*}$p$<$0.1; $^{**}$p$<$0.05; $^{***}$p$<$0.01} \\ 
\end{tabular} 
\end{table}

\begin{table}[!htbp] \centering 
  \caption{Effect of difference between stimuli slopes on response's distance from mathematical average of stimuli slopes} 
  \label{} 
\begin{tabular}{@{\extracolsep{5pt}}lD{.}{.}{-3} } 
\\[-1.8ex]\hline 
\hline \\[-1.8ex] 
 & \multicolumn{1}{c}{\textit{Dependent variable:}} \\ 
\cline{2-2} 
\\[-1.8ex] & \multicolumn{1}{c}{Distance from mathematical average} \\ 
\hline \\[-1.8ex] 
 Difference in stimuli slopes & 0.171^{***} \\ 
  & (0.031) \\ 
  Constant & -0.025 \\ 
  & (0.025) \\ 
 \hline \\[-1.8ex] 
Observations & \multicolumn{1}{c}{1,133} \\ 
R$^{2}$ & \multicolumn{1}{c}{0.026} \\ 
Adjusted R$^{2}$ & \multicolumn{1}{c}{0.025} \\ 
\hline 
\hline \\[-1.8ex] 
\textit{Note:}  & \multicolumn{1}{r}{$^{*}$p$<$0.1; $^{**}$p$<$0.05; $^{***}$p$<$0.01} \\ 
\end{tabular} 
\end{table}

\begin{table}[!htbp] \centering 
  \caption{Effect of difference between stimuli slopes on response's distance from mathematical average of stimuli slopes - accounting for priors} 
  \label{} 
\begin{tabular}{@{\extracolsep{5pt}}lD{.}{.}{-3} } 
\\[-1.8ex]\hline 
\hline \\[-1.8ex] 
 & \multicolumn{1}{c}{\textit{Dependent variable:}} \\ 
\cline{2-2} 
\\[-1.8ex] & \multicolumn{1}{c}{Distance from mathematical average} \\ 
\hline \\[-1.8ex] 
 Difference in stimuli slopes & 0.219^{***} \\ 
  & (0.035) \\ 
  Prior & 0.268^{***} \\ 
  & (0.037) \\ 
  Constant & -0.138^{***} \\ 
  & (0.030) \\ 
 \hline \\[-1.8ex] 
Observations & \multicolumn{1}{c}{839} \\ 
R$^{2}$ & \multicolumn{1}{c}{0.098} \\ 
Adjusted R$^{2}$ & \multicolumn{1}{c}{0.096} \\ 
\hline 
\hline \\[-1.8ex] 
\textit{Note:}  & \multicolumn{1}{r}{$^{*}$p$<$0.1; $^{**}$p$<$0.05; $^{***}$p$<$0.01} \\ 
\end{tabular} 
\end{table} 

\begin{table}[!htbp] \centering 
  \caption{Effect of difference between stimuli slopes on response's distance from the first stimuli slope} 
  \label{} 
\begin{tabular}{@{\extracolsep{5pt}}lD{.}{.}{-3} } 
\\[-1.8ex]\hline 
\hline \\[-1.8ex] 
 & \multicolumn{1}{c}{\textit{Dependent variable:}} \\ 
\cline{2-2} 
\\[-1.8ex] & \multicolumn{1}{c}{Distance from first stimuli} \\ 
\hline \\[-1.8ex] 
 Difference in stimuli slopes & -0.096^{*} \\ 
  & (0.052) \\ 
  Constant & 0.567^{***} \\ 
  & (0.041) \\ 
 \hline \\[-1.8ex] 
Observations & \multicolumn{1}{c}{1,133} \\ 
R$^{2}$ & \multicolumn{1}{c}{0.003} \\ 
Adjusted R$^{2}$ & \multicolumn{1}{c}{0.002} \\ 
\hline 
\hline \\[-1.8ex] 
\textit{Note:}  & \multicolumn{1}{r}{$^{*}$p$<$0.1; $^{**}$p$<$0.05; $^{***}$p$<$0.01} \\ 
\end{tabular} 
\end{table} 

\begin{table}[!htbp] \centering 
  \caption{Effect of difference between stimuli slopes on response's distance from the stronger slope stimuli} 
  \label{} 
\begin{tabular}{@{\extracolsep{5pt}}lD{.}{.}{-3} } 
\\[-1.8ex]\hline 
\hline \\[-1.8ex] 
 & \multicolumn{1}{c}{\textit{Dependent variable:}} \\ 
\cline{2-2} 
\\[-1.8ex] & \multicolumn{1}{c}{Distance from stronger slope stimuli} \\ 
\hline \\[-1.8ex] 
 Difference in stimuli slopes & -0.524^{***} \\ 
  & (0.048) \\ 
  Constant & 0.990^{***} \\ 
  & (0.038) \\ 
 \hline \\[-1.8ex] 
Observations & \multicolumn{1}{c}{1,133} \\ 
R$^{2}$ & \multicolumn{1}{c}{0.095} \\ 
Adjusted R$^{2}$ & \multicolumn{1}{c}{0.094} \\ 
\hline 
\hline \\[-1.8ex] 
\textit{Note:}  & \multicolumn{1}{r}{$^{*}$p$<$0.1; $^{**}$p$<$0.05; $^{***}$p$<$0.01} \\ 
\end{tabular} 
\end{table} 

\begin{table}[!htbp] \centering 
  \caption{Effect of absolute stimuli slope values on the response's distance from the larger slope} 
  \label{} 
\begin{tabular}{@{\extracolsep{5pt}}lD{.}{.}{-3} } 
\\[-1.8ex]\hline 
\hline \\[-1.8ex] 
 & \multicolumn{1}{c}{\textit{Dependent variable:}} \\ 
\cline{2-2} 
\\[-1.8ex] & \multicolumn{1}{c}{Distance from larger slope} \\ 
\hline \\[-1.8ex] 
 Larger Slope & 0.283^{***} \\ 
  & (0.022) \\ 
  Smaller Slope & -0.280^{***} \\ 
  & (0.050) \\ 
  Age & -0.001 \\ 
  & (0.001) \\ 
  Gender (Female) & 0.018 \\ 
  & (0.118) \\ 
  Gender (Male) & 0.009 \\ 
  & (0.118) \\ 
  Score (Attitude towards science and scientists) & 0.003 \\ 
  & (0.004) \\ 
  Score (Visual literacy) & 0.004 \\ 
  & (0.003) \\ 
  Constant & -0.822^{***} \\ 
  & (0.153) \\ 
 \hline \\[-1.8ex] 
Observations & \multicolumn{1}{c}{1,141} \\ 
R$^{2}$ & \multicolumn{1}{c}{0.165} \\ 
Adjusted R$^{2}$ & \multicolumn{1}{c}{0.160} \\ 
\hline 
\hline \\[-1.8ex] 
\textit{Note:}  & \multicolumn{1}{r}{$^{*}$p$<$0.1; $^{**}$p$<$0.05; $^{***}$p$<$0.01} \\ 
\end{tabular} 
\end{table}

\begin{figure*}[t!]
\setlength{\textfloatsep}{4pt plus 1.0pt minus 1.0pt}
\setlength{\intextsep}{4pt plus 1.0pt minus 1.0pt}
\setlength{\floatsep}{4pt plus 1.0pt minus 1.0pt}
\setlength{\dbltextfloatsep}{6pt plus 1.0pt minus 2.0pt}
\setlength{\dblfloatsep}{6pt plus 1.0pt minus 2.0pt}
\centering
  \includegraphics[width=\linewidth]{Figures_Supplmentary/cropped_SupplementaryMaterials_addedLines_moreVarName_moreSpace_bigger_text_new_new_new_esponseSlope_compuedSlope_density.pdf}
  \caption{Position of stimuli and response slopes on an absolute slope scale (x-axis). The number on the top right corner denotes the Condition number for easy reference. Note: The x-axis has been rescaled by a factor of 0.1 for Experiments 2B and 3 for easy visual comparison. The left panel shows the Conditions that contains a high negative slope, while the right panel shows the Conditions that contains a high positive slope.}
    \label{fig:errorBars}
\end{figure*}

% Flowchart figure
\begin{figure*}[h!]
\centering
  \includegraphics[width = \linewidth]{Figures_June24/Flowchart_v1_powerpoint.pdf}
  \caption{A schematic of the experiment flow}
    \label{fig:schematicExperiment}
\end{figure*}

\end{document}
